# Supplementary material for: Theory of momentum-resolved phonon spectroscopy in the electron microscope
Source: arXiv:1804.10475 ancillary file (2019-04-05)
Supplement: Supplementary file 1 [file RNicholls_letter_SM.pdf]

# Theory of momentum-resolved phonon spectroscopy in the electron microscope

R.J. Nicholls,<sup>1</sup> F.S. Hage,<sup>2</sup> D.G. McCulloch,<sup>3</sup> Q.M. Ramasse,<sup>4,5</sup> K. Refson,<sup>6,7</sup> and J.R. Yates<sup>1</sup>

<sup>1</sup>*Department of Materials, University of Oxford, Parks Road, Oxford, OX1 3PH, United Kingdom*

<sup>2</sup>*SuperSTEM Laboratory, SciTech Daresbury Campus,  
Keckwick Lane, Warrington, WA4 4AD, United Kingdom*

<sup>3</sup>*Physics, School of Science, RMIT University, Melbourne, VIC 3001, Australia*

<sup>4</sup>*SuperSTEM Laboratory, SciTec Daresbury Campus,  
Keckwick Lane, Warrington, WA4 4AD, United Kingdom*

<sup>5</sup>*School of Physics and School of Chemical and Process Engineering,  
University of Leeds, Leeds LS2 9JT, United Kingdom*

<sup>6</sup>*Department of Physics, Royal Holloway, University of London, Egham TW20 0EX, United Kingdom*

<sup>7</sup>*ISIS Spallation Neutron Source, RAL, Chilton, Didcot OX11 0QX, United Kingdom*

## COMMENTS ON RELATED TREATMENTS

Electrons have been used to probe phonons in a reflection geometry since the 1960s [1, 2]. The geometrical constraints in that case mean that the theoretical treatments used are not applicable to transmission electron energy loss spectroscopy (EELS). For the transmission geometry, two different scattering regimes have been identified by Dwyer *et al.* [3]: dipole scattering and localised vibrational scattering. Dipole scattering involves small momentum transfer and Radtke *et al.* [4] have used density functional theory to model EEL spectra in this regime. To interpret momentum dependent spectra, we are interested in the localised vibrational scattering regime.

Rez [5] obtained an expression for the differential cross-section in the case of a fast electron interacting with a stretch vibration in a diatomic molecule and there are clear similarities between his equation for that specific case and our general equation. Rez commented on the implications of the  $\mathbf{q} \cdot \mathbf{e}(\mathbf{q}_0, j)$  term and also pointed out the connection between the cross section and the loss function (the imaginary part of  $-1/\epsilon(E, \mathbf{q})$  where  $\epsilon(E, \mathbf{q})$  is the energy and wavevector-dependent dielectric function); more details of the relationship can be found in reference [6]. Saavedra and Javier García de Abajo [7] derived an expression for the case of a fast electron interacting with nanographene and made the connection between the density of vibrational states and EEL spectra which is implicit in our approach. Forbes and Allen [8] have used a transition potential approach to calculate phonon EEL spectra from a plane wave and a focused coherent probe. Hohenester *et al.* [9, 10] have used a local dielectric description to interpret the  $q = 0$  spectrum for a nanocube using the phonon modes across the whole Brillouin Zone.

## SCATTERING FACTOR FORMALISM FOR NEUTRONS AND X-RAY

For X-Rays, the double differential cross section for energy loss can be written as [11, 12]

$$\frac{d^2\sigma}{d\Omega dE_1} = \frac{e^4}{m^2 c^4} \frac{k_1}{k_0} |\epsilon_0^* \cdot \epsilon_1|^2 S(\mathbf{q}, \omega) \quad (1)$$

where  $\epsilon_0$  and  $\epsilon_1$  are the polarisation vectors of the incoming and outgoing photons. The scattering function,  $S(\mathbf{q}, \omega)$  is given by

$$S(\mathbf{q}, \omega) = \left| \sum_i f_i(\mathbf{q}) e^{-W_i} [\mathbf{q} \cdot \mathbf{e}(\mathbf{q}_0, j)] M_i^{-1/2} e^{i\mathbf{q} \cdot \mathbf{r}} \right|^2 \frac{< n_{\mathbf{q}_0 j} + 1 >}{\omega_{\mathbf{q}_0 j}} \delta(\omega - \omega_{\mathbf{q}_0 j}) \quad (2)$$

To obtain the neutron scattering function, the atomic form factor is replaced by the Fermi scattering length,  $b$  [11, 13].

## EXPERIMENTAL DETAILS

Based on earlier experimental procedures for acquiring momentum resolved core and valance EEL spectra in the (scanning) transmission electron microscope ((S)TEM) (see e.g. Refs. [14, 15] and references therein), we use the electromagnetic scan coils of the STEM to accurately control the range, magnitude and direction of momentum transfers accepted by the circular spectrometer entrance aperture. Thus our momentum resolved spectra are acquired serially [15], rather than in parallel [14]. By carefully balancing the simultaneously achievable spatial and momentum resolutions, we probe phonon dispersions along high symmetry directions of the first Brillouin zones of hBN and cBN, using a  $\sim 1nm$  electron probe, a momentum resolution  $\Delta q = \pm 0.5 \text{\AA}^{-1}$  and an energy resolution  $\Delta E = 18-40 meV$  (increasing with increasing  $q$ ) [16].

All experimental work was carried out on a Nion UltraSTEM100MC dedicated STEM [17], equipped with a Gatan Enfium EEL ERS spectrometer (optimised with high stability electronics). The microscope was operated at an acceleration voltage of 60kV, in order to minimise electron beam induced irradiation damage. No post-acquisition de-noising or deconvolution routines were used for any experimental spectrum. In each spectrum shown in Figure 1 in the main text and Figures S1 and S2 in the Supplemental material, the zero loss peak (ZLP) tail contribution was subtracted by fitting a power law function over an energy loss window preceding the lowest energy loss peak.

In inelastic neutron spectroscopy, it is necessary to determine the full resolution ellipsoid, expressing energy and momentum resolutions in terms of energy loss and momentum transfer [18]. In our case, the momentum resolution

( $\Delta q = \pm 0.5 \text{\AA}^{-1}$ ) is limited by beam convergence and spectrometer acceptance angles (both with a half-angle of  $3 \text{ mrad}$ ), while the energy resolution ( $\Delta E$ ) is approximately constant as a function of momentum transfer. Experimentally,  $\Delta E$  is measured as the full width at half maximum (FWHM) of the quasi elastic ZLP. Due primarily to instrumental instabilities, along with electron-atom Compton scattering [19], the measured ZLP FWHM effectively increases from  $18-20 \text{ meV}$  (near the optical limit) to  $30-40 \text{ meV}$  for larger momentum transfers. The ZLP broadening due to instrumental instabilities increases with  $q$  due to the significantly longer exposure times required at higher  $q$  (from  $0.1 \text{ s}$  near the  $\Gamma$  point up to  $90 \text{ s}$  at the Brillouin zone boundaries). In light of the above mentioned factors, the more involved procedure for determining the full resolution ellipsoid [18] was not deemed appropriate. For a more detailed discussion of the experimental procedure and associated parameters, see reference [16].

## DETAILS OF FIRST-PRINCIPLES CALCULATIONS

The phonon eigenvalues and dispersions have been calculated with density functional theory code CASTEP [20] using norm-conserving pseudopotentials and the PBE exchange-correlation functional. A geometry optimisation was first carried out on both crystal structures using a cut-off energy of  $850 \text{ eV}$ , a k-point sampling of  $2\pi \times 0.03 \text{\AA}^{-1}$  and the structures were optimised until the forces on each atom did not exceed  $0.001 \text{ eV/\AA}$ . Phonon dispersions were then calculated using density functional perturbation theory (DFPT) with Fourier interpolation used to calculate the dynamical matrices on a finer grid [21]. The DFPT calculations used a cut-off energy of  $850 \text{ eV}$ , a k-point spacing of  $2\pi \times 0.03 \text{\AA}^{-1}$ , a phonon k-point spacing of  $2\pi \times 0.07 \text{\AA}^{-1}$  and a fine phonon k-point path spacing of at most  $2\pi \times 0.05 \text{\AA}^{-1}$ . The numerical parameters were all carefully checked so that their value did not influence the final phonon dispersions.

## ATOMIC FORM FACTOR

The atomic form factor has been included using [22]

$$f(q) = \sum_i a_i \exp\left(-b_i \left(\frac{q}{4\pi}\right)^2\right) + c \quad (3)$$

| atom | $a_1$   | $b_1$   | $a_2$  | $b_2$  | $a_3$  | $b_3$   | $a_4$  | $b_4$  | c       |
|------|---------|---------|--------|--------|--------|---------|--------|--------|---------|
| B    | 2.0545  | 23.2185 | 1.3326 | 1.021  | 1.0979 | 60.3498 | 0.7068 | 0.1403 | -0.1932 |
| N    | 12.2126 | 0.0057  | 3.1322 | 9.8933 | 2.0125 | 28.9975 | 1.1663 | 0.5826 | -11.529 |

The quantity  $f_{atom}(\mathbf{q})$  used in the main paper is equal to  $-ef(q)$ .

## DEBYE-WALLER FACTOR

The Debye-Waller factor for a particular atom and a specific value of  $\mathbf{q}$  is given by [23]:

$$e^{-2W} = e^{-\langle (\mathbf{q} \cdot \mathbf{u})^2 \rangle} = e^{-2\pi^2 \sum_i (q_i^2 U^{ii})} \quad (4)$$

where the sum over  $i$  represents the sum over the three reciprocal lattice directions. The values for  $U^{ii}$  are the mean-squared displacement values calculated by CASTEP using the definition in [23]. The off-diagonal components  $U^{ji}$  are zero for both cBN and hBN, producing the simplified version of the Debye-Waller factor above.

The  $U^{ii}$  values are dependent on temperature. To get an idea of the variation with temperature, the  $U^{ii}$  for cBN are listed in Table S1 for temperatures between  $293$  and  $303 \text{ K}$ . The  $U^{ii}$  values calculated at  $293 \text{ K}$  have been used for the boron nitride simulation included in this paper.

| Temperature (K) | Atom | $U^{11}$ | $U^{22}$ | $U^{33}$ |
|-----------------|------|----------|----------|----------|
| 293.0           | B    | 0.068874 | 0.068874 | 0.068874 |
| 293.0           | N    | 0.068341 | 0.068341 | 0.068341 |
| 294.8           | B    | 0.069291 | 0.069291 | 0.069291 |
| 294.8           | N    | 0.068756 | 0.068756 | 0.068756 |
| 297.5           | B    | 0.069916 | 0.069916 | 0.069916 |
| 297.5           | N    | 0.069379 | 0.069379 | 0.069379 |
| 301.2           | B    | 0.070750 | 0.070750 | 0.070750 |
| 301.2           | N    | 0.070211 | 0.070211 | 0.070211 |
| 303.0           | B    | 0.071166 | 0.071166 | 0.071166 |
| 303.0           | N    | 0.070626 | 0.070626 | 0.070626 |

TABLE S1. Variation in  $U^{ii}$  with temperature for cBN.

### MOMENTUM RESOLVED CUBIC BORON NITRIDE DATA: $\Gamma - K$

Experimental and simulated data for cBN along the  $\Gamma - K$  direction in reciprocal space are shown in Figure S1a. The corresponding part of the phonon dispersion curve showing the contributions of the different modes is shown in Figure S1c. In this case, four of the branches contribute to the EEL spectra. Unlike the  $\Gamma - X$  case, the lower energy mode dominates at higher values of  $q$  so that the EEL spectrum appears to shift as you move across the Brillouin zone.

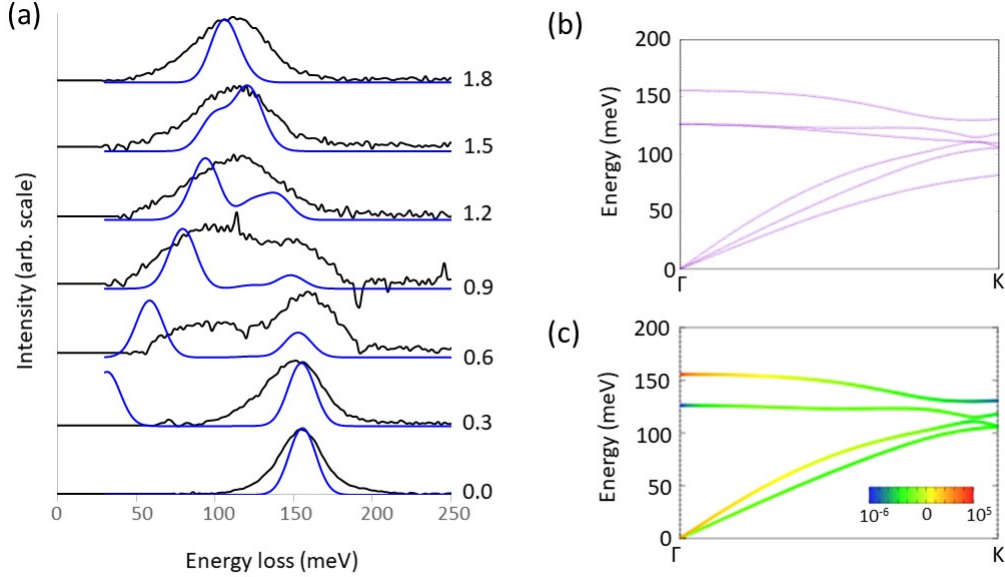

FIG. S1. Experimental and simulated phonon EEL spectra for cBN in the  $\Gamma - K$  direction in reciprocal space (a) (Each spectrum is labelled by the corresponding  $q$  vector in units of  $\text{\AA}^{-1}$ , given to one decimal place.) The corresponding section of the phonon dispersion showing all the bands (b) and the intensities of the contributing phonon branches on a  $\log_{10}$  scale (c).

### MOMENTUM RESOLVED HEXAGONAL BORON NITRIDE DATA: $\Gamma - M$

Experimental and simulated data for hBN along the  $\Gamma - M$  direction in reciprocal space are shown in Figure S2a. The corresponding part of the phonon dispersion curve showing the contributions of the different modes is shown in Figure S2c. As with the  $\Gamma - K$  direction, four branches contribute towards the spectrum. In this case the lower two branches are almost the same energy across most of the Brillouin zone. These two branches are unaffected by LO-TO splitting [24] unlike the upper two branches. The simulations include LO-TO splitting in the case of an infinite crystal and overestimate the energy of the upper branch for a crystal of the thickness used in these experiments. As with the  $\Gamma - K$  direction, the discrepancy between simulation and experiment is likely to be due to the way LO-TO splitting is

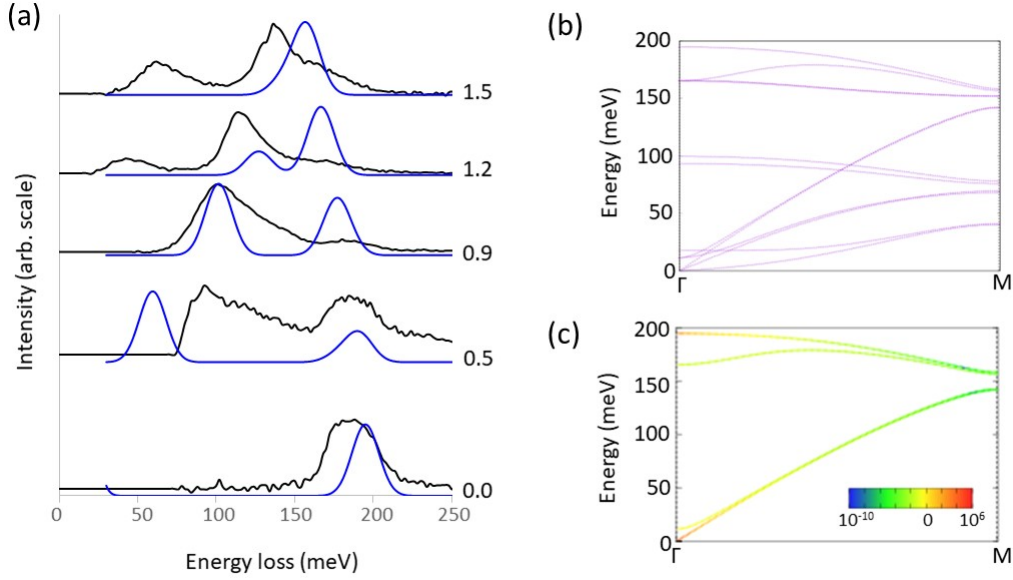

FIG. S2.

Experimental and simulated phonon EEL spectra for hBN in the  $\Gamma - M$  direction in reciprocal space (a). (Each spectrum is labelled by the corresponding  $q$  vector in units of  $\text{\AA}^{-1}$ , given to one decimal place.) The corresponding section of the phonon dispersion showing all the bands (b) and the intensities of the contributing phonon branches on a  $\log_{10}$  scale (c). Note: the  $0.0\text{-}0.9\text{\AA}^{-1}$  and  $1.2\text{-}1.5\text{\AA}^{-1}$  data sets have been acquired from different hBN flakes.

included in the simulation and the experimental geometry, including the finite momentum resolution and the spatial resolution of the experiment. As in the  $\Gamma - K$  case, the effect of the curvature of the Ewald Sphere can also be seen with low energy out-of-plane modes contributing at large values of  $q$ .

## CHARGE TRANSFER

The charge calculated from a Mulliken population analysis is used to account for the charge transfer within the material. The values were taken from the CASTEP calculations:  $0.64e$  and  $-0.64e$  for the boron and nitrogen atoms in cBN and  $0.82e$  and  $-0.82e$  for the boron and nitrogen atoms in hBN. Including the charge transfer essentially changes how much the nuclear term is screened by the electronic term in the Hamiltonian and it alters the relative intensities of the different modes, in particular including the charge transfer damps the contribution from the lower energy modes at small  $q$  and reduces the contribution from the higher energy modes at large  $q$ . Figure S3 shows spectra for the  $\Gamma - X$  direction in cBN simulated with and without including the effects of charge transfer. Including charge transfer leads to a better visual match with the experimental intensities of the modes. Figure S4 shows spectra for the  $\Gamma - K$  direction in hBN with and without including the effects of charge transfer. Although this case is more complicated due to the contributions from out-of-plane modes in the experimental data, including the effects of charge transfer in the simulations produces a better match with experiment.

- 
- [1] F. M. Propst and T. C. Piper, *Journal of Vacuum Science and Technology* **4**, 53 (1967).
  - [2] H. Ibach and D. L. Mills, *Electron Energy Loss Spectroscopy and Surface Vibrations* (Academic Press, 1982).
  - [3] C. Dwyer, T. Aoki, P. Rez, S. L. Y. Chang, T. C. Lovejoy, and O. L. Krivanek, *Physical Review Letters* **117**, 256101 (2016).
  - [4] G. Radtke, D. Taverna, M. Lazzeri, and E. Balan, *Physics Review Letters* **119**, 027402 (2017).
  - [5] P. Rez, *Microsc. Microanal.* **20**, 671 (2014).
  - [6] K. Sturm, *Z. Naturforsch.* **48a**, 233 (1993).
  - [7] J. R. M. Saavedra and J. G. de Abajo, *Physical Review B* **92**, 115449 (2015).
  - [8] B. D. Forbes and L. J. Allen, *Physical Review B* **94**, 014110 (2016).

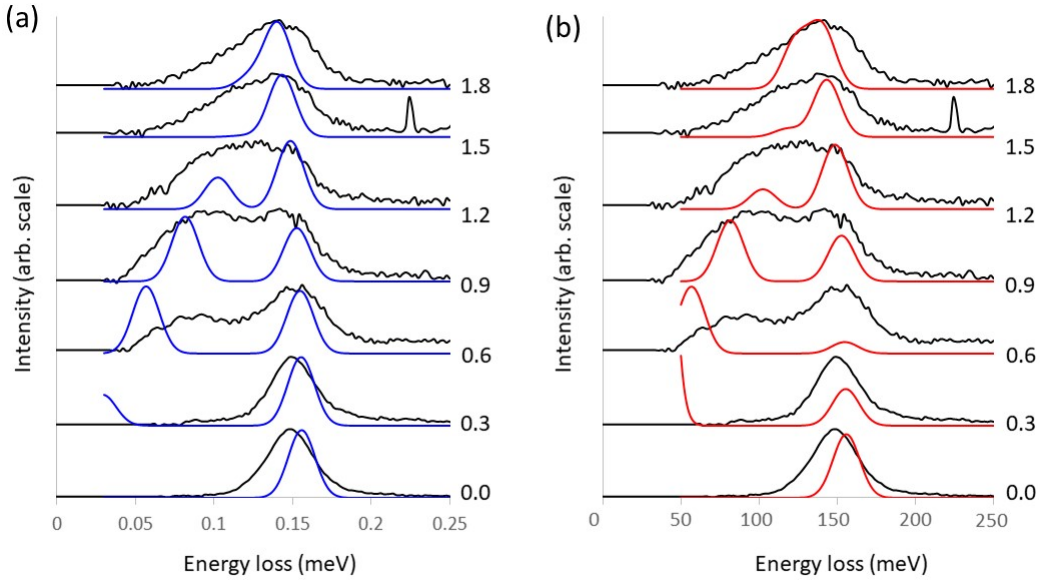

FIG. S3. Spectra simulated for the  $\Gamma - X$  direction in cBN with (a) and without (b) the effects of charge transfer included. Each spectrum is labelled by the corresponding  $q$  vector in units of  $\text{\AA}^{-1}$ , given to one decimal place.

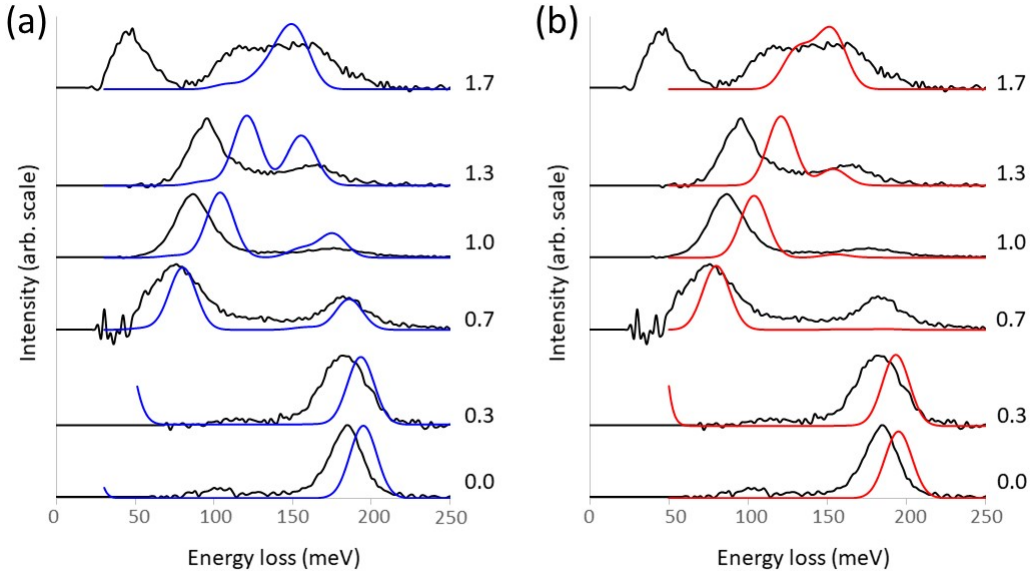

FIG. S4. Spectra simulated for the  $\Gamma - K$  direction in hBN with (a) and without (b) the effects of charge transfer included. Each spectrum is labelled by the corresponding  $q$  vector in units of  $\text{\AA}^{-1}$ , given to one decimal place.

- [9] M. J. Lagos, A. Trügler, U. Hohenester, and P. E. Batson, *Nature* **543**, 529 (2017).
- [10] U. Hohenester, A. Trügler, P. E. Batson, and M. J. Lagos, *Physical Review B* **97**, 165418 (2018).
- [11] E. Burkel, *J. Phys.: Condens. Matter* **13**, 7627 (2001).
- [12] S. K. Sinha, *J. Phys.: Condens. Matter* **13**, 7511 (2001).
- [13] G. L. Squires, *Introduction to the theory of Thermal Neutron Scattering* (Cambridge University Press, 2012).
- [14] R. D. Leapman, P. L. Fejes, and J. Silcox, *Physical Review B* **28**, 2361 (1983).
- [15] F. S. Hage, Q. M. Ramasse, D. M. Kepaptsoglou, Ø. Prytz, A. E. Gunnaes, G. Helgesen, and R. Brydson, *Physical Review B* **88**, 155408 (2013).
- [16] F. S. Hage, R. J. Nicholls, J. R. Yates, D. MuCulloch, T. C. Lovejoy, N. Delby, O. L. Krivanek, K. Refson, and Q. M. Ramasse, in preparation.

- [17] O. L. Krivanek, J. P. Ursin, N. J. Bacon, G. J. Corbin, N. Dellby, P. Hrnčirik, M. F. Murfitt, C. S. Own, and S. Szilagy, Philosophical Transactions of the Royal Society of London A: Mathematical, Physical and Engineering Sciences **367**, 3683 (2009).
- [18] L. D. Cussen, Journal of Applied Crystallography **35**, 615 (2002).
- [19] G. Argentero, C. Mangler, J. Kotakoski, F. R. Eder, and J. C. Meyer, Ultramicroscopy **151**, 23 (2015).
- [20] S. J. Clark, M. D. Segall, C. J. Pickard, P. J. Hasnip, M. J. Probert, K. Refson, and M. Payne, Z. Kristall. **220**, 567 (2005).
- [21] K. Refson, P. R. Tulip, and S. J. Clark, Phys. Rev. B **73**, 155114 (2006).
- [22] P. J. Brown, A. G. Fox, E. N. Maslen, M. A. O’Keefe, and B. T. M. Willis, *International Tables for Crystallography*, Vol. C (2006) Chap. 6.1.
- [23] K. N. Trueblood, H.-B. Burgi, H. Burzlaff, J. D. Dunitz, C. M. Gramaccioli, H. H. Schulz, U. Shmueli, and S. C. Abrahams, Acta Cryst. **A52**, 770 (1996).
- [24] K. H. Michel and B. Verberck, Physical Review B **83**, 115328 (2011).
